# Supplementary material for: Self-Optimizing Feature Transformation
Source: arXiv:2209.08044 source file (2022-12-23)
Supplement: Supplementary file 1 [file appendix.tex]

\newpage

\begin{center}
\textbf{\fontfamily{ppl} \fontsize{13}{0}\selectfont
Appendix
}%
\bigskip
\end{center}

\noindent\textbf{Pseudo-code.} Algorithm ~\ref{grfg_alg} illustrates the pseudo-code of our feature generation framework, which aids readers in comprehending our method.
Specifically, at each iteration, we first cluster the feature set into different feature groups by M-Clustering algorithm.
Then, we utilize the feature group agent1, operation agent, and feature group agent2 to select feature groups and operations in a cascading cooperation way.
After that, we generate new features by applying the selected operation to selected feature groups.
During the generation process, we use relevance prioritized generation strategies to generate meaningful features by  selecting the most distinct features from two feature groups.
Moreover, we combine the generated features and original feature set together to form a new feature set and adopt a downstream task to validate its performance.
If the performance is larger than the optimal feature set, we need to replace the optimal one with the current one.
In addition, we calculate the reward signal of each agent and store the experiences data into replay buffers for updating the parameters of agents.
Following that, we will conduct the feature selection to control the size of generated new feature set and replace it as the initial feature set at the next iteration.
Finally, when the iteration process ends up, we return the optimal feature set that maximizes the performance of the downstream task.

\noindent\textbf{Demo.} 
To observe the exploration process of GRFG conveniently, we develop a web demo to monitor the changes in the performance of the downstream task.
Figure ~\ref{fig:demo} shows the interface of the demo for monitoring a classification task.
We use four windows to display the changes of Accuracy, Precision, Recall, and F1 Score of the downstream task.
In each window, there are three lines: i) Best, which is used to record the best performance during the iterative feature generation process; ii) Base, which is utilized to show the basic performance of the original feature space; iii) and GRFG, which is employed to record the exploration process of our method. 
We can see that  compared with the Base line, GRFG helps the machine learning model discover an optimal feature space that significantly improves the performance of the downstream task.

\begin{figure*}[!t]
    \centering
    \includegraphics[width=0.85\linewidth]{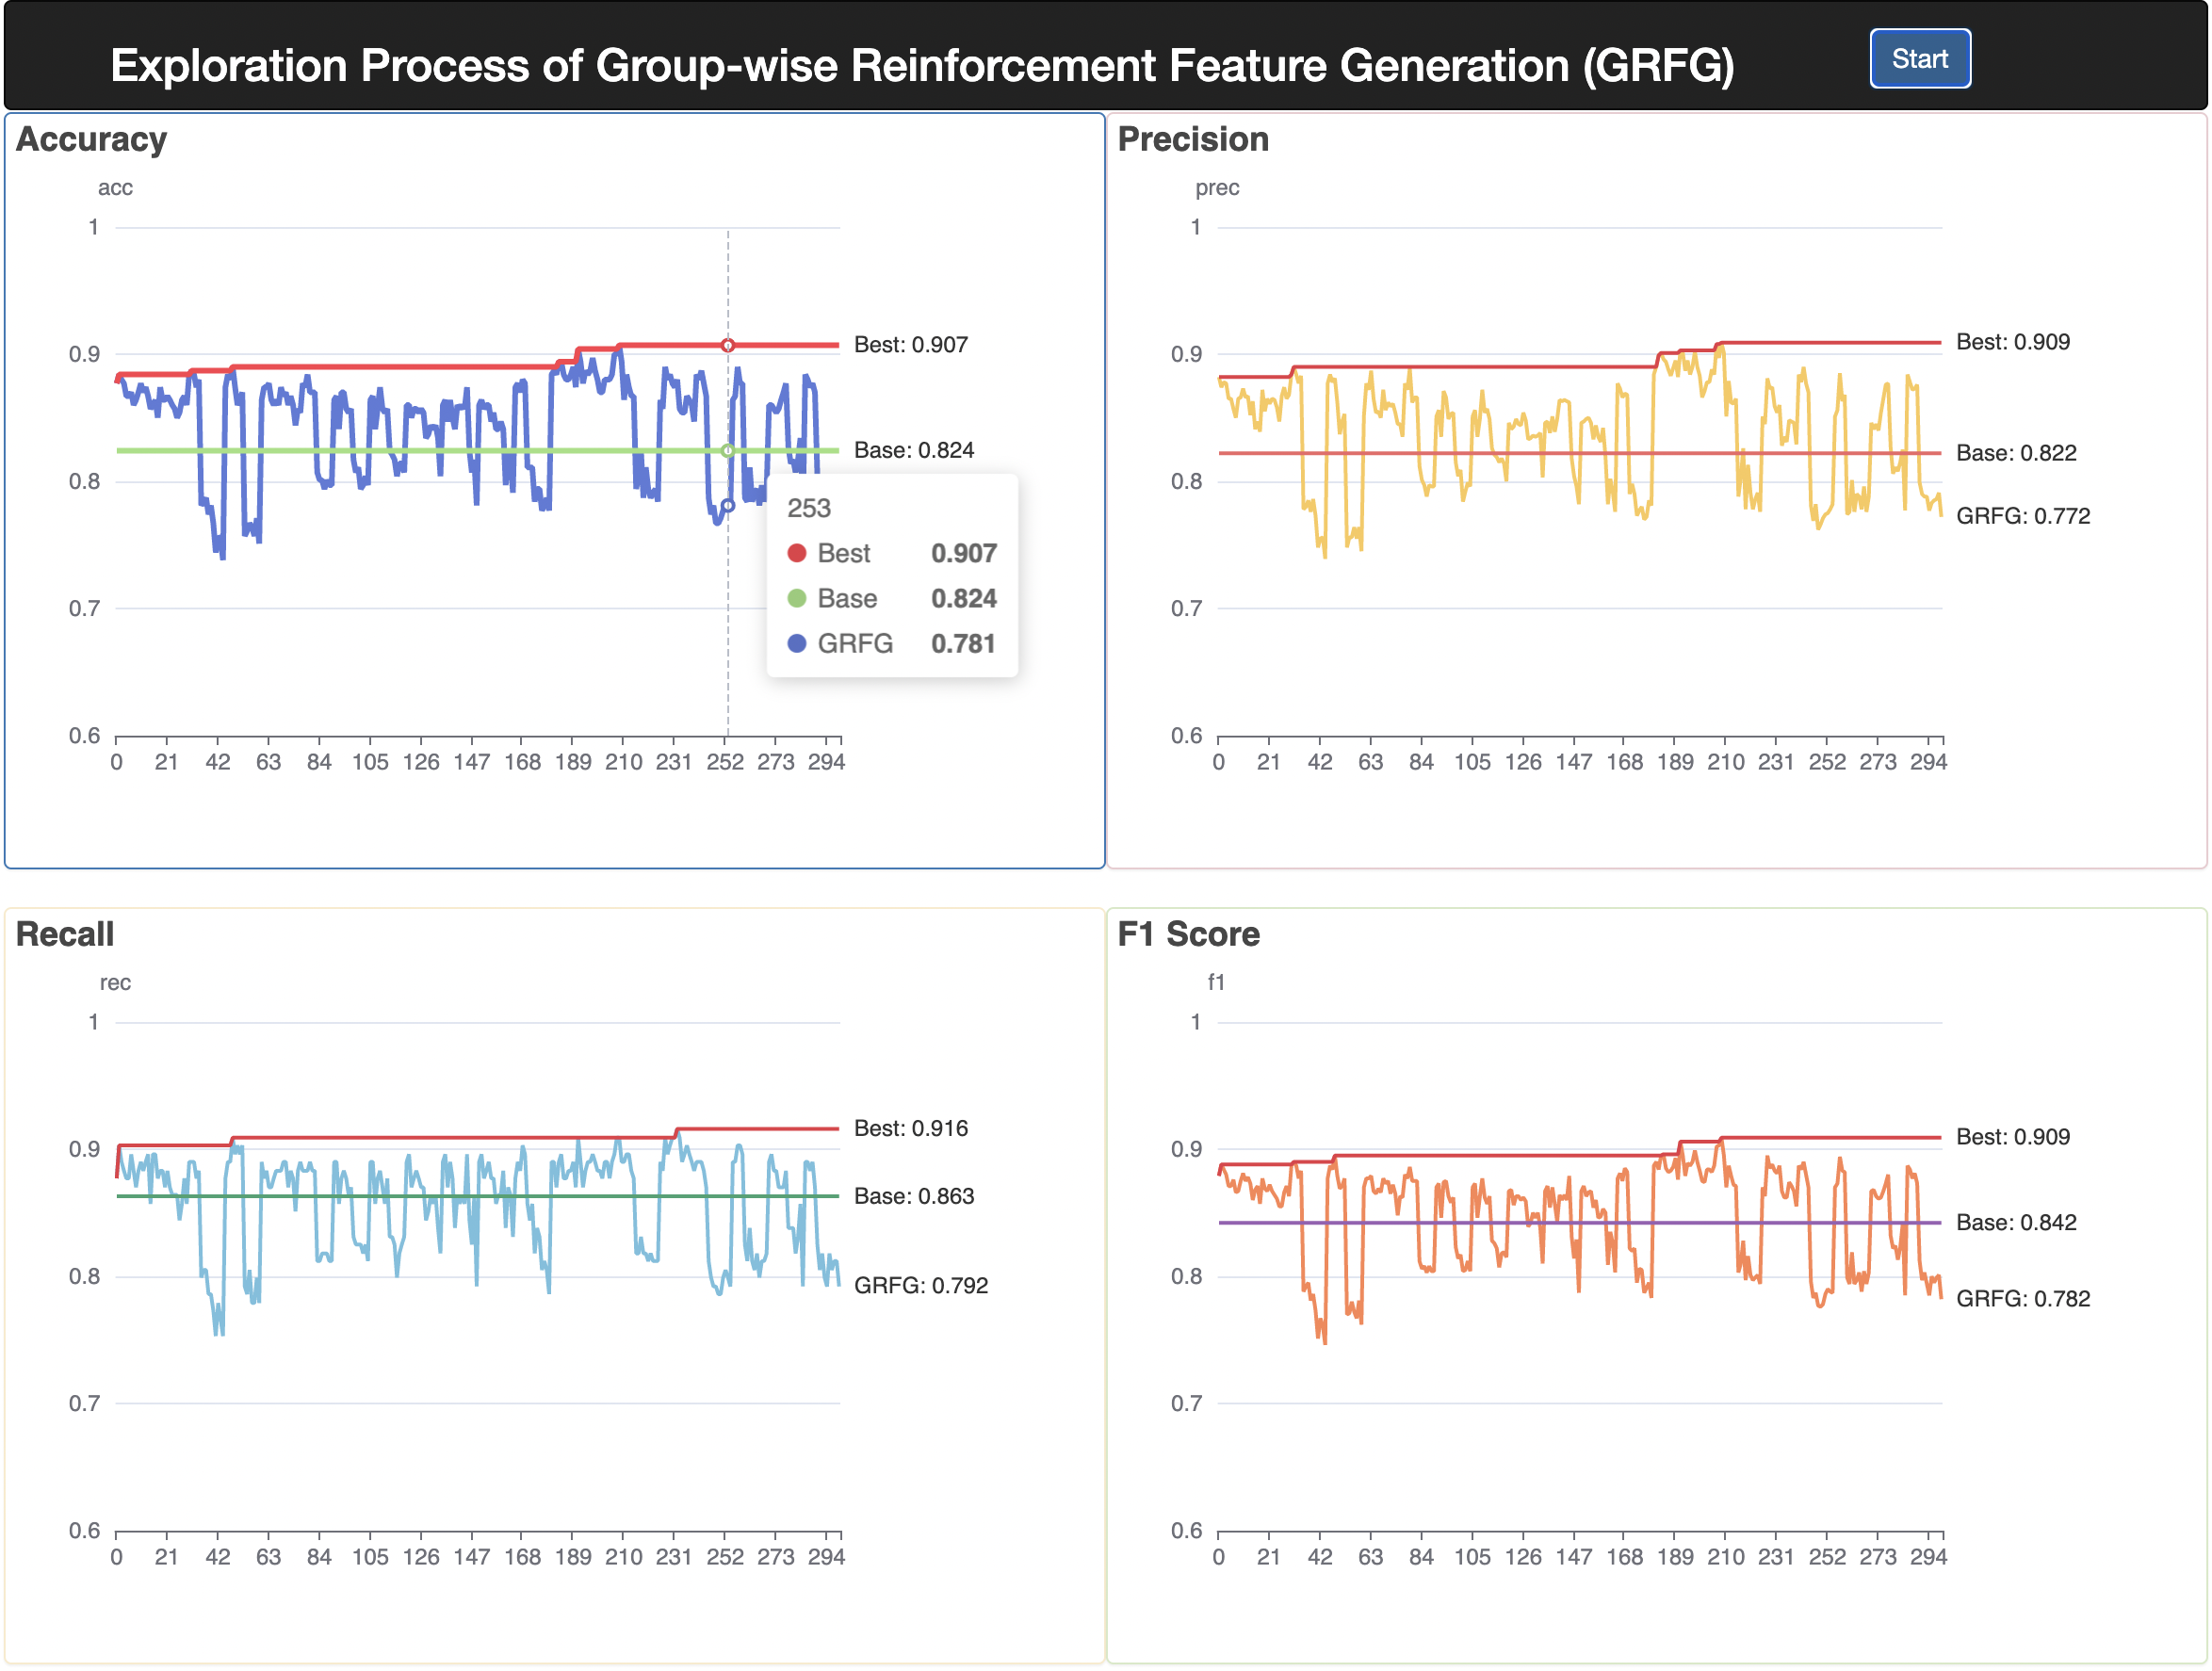}
    \vspace{-0.1cm}
    \captionsetup{justification=centering}
    \vspace{-0.1cm}
    \caption{Demo for monitoring the exploration process of GRFG. 
    }
    \vspace{-0.5cm}
    \label{fig:demo}
\end{figure*}

\begin{algorithm}
	\SetAlgoNoLine
	\LinesNumbered
% 	\SetKwInOut{Input}{Input}\SetKwInOut{Output}{Output}
% 	\Input{Original feature set $\mathcal{F}_0$, label $y$, operation set $\mathcal{O}$, episode number $N_e$, step number in each episode $N_s$, maximize size multiple $M_{max}$, minimize size multiple $M_{min}$.}
	\SetKwInOut{Input}{Input}\SetKwInOut{Output}{Output}
	\Input{Original feature set $\mathcal{F}$, label $y$, operation set $\mathcal{O}$, feature groups $\mathcal{C}$ , epoch number $N_e$, iteration number per epoch $N_i$, feature size tolerance threshold $M_{max}$, the downstream task performance indicator $V_A$.}
	\Output{Optimal generated feature set $\mathcal{F}^{*}$.}
	
	Initialize three reinforcement learning agents, and initialize each agent's replay memory $\{\mathcal{D}^1, \mathcal{D}^o, \mathcal{D}^2\}$, $Q$-value function $\{Q^1, Q^o, Q^2\}$;\\
	Initialize $\mathcal{F}^{*}$ = $\mathcal{F}$.\\
	\For{$i = 1~to~N_e$}{
 	Initialize $\mathcal{F}_{i}$ = $\mathcal{F}$;\\
 	$\mathcal{C}$ = M-Clustering($\mathcal{F}_i$);\\
	\For{$t= 1~ to~N_i$}
	    {   Derive $s^1_t = Rep(\mathcal{F}_{i,t})$;\\
	   % Initialize $\mathcal{F}_g$ = $\mathcal{F}_0$;
	        Select one meta feature group by:
	        $\mathcal{C}_t^1 = a^1_{t}= \text{argmax}_a Q^1(s^1_t,a)$;\\
	        Derive $s^o_{t} = Rep(\mathcal{F}_{i,t}) \oplus Rep(\mathcal{C}^1_t)$;\\
	        Select operation $o_t$ by:
	        $o_t = a^o_{t}= \text{argmax}_a Q^o(s^o_t,a)$;\\
	        Derive $s^2_t = Rep(\mathcal{F}_{0,t}) \oplus Rep(\mathcal{C}^1_t) \oplus Rep(o_t)$;\\
	        Select the second meta feature by:
	        $\mathcal{C}^2_t = a^2_{t} = \text{argmax}_a Q^2(s^2_t,a)$;\\
	        Generate new features $\mathcal{F}^g_t$ by applying $o_t$ to  $\mathcal{C}_t^1$ and $\mathcal{C}_t^2$ based on  prioritized  generation strategies;\\
	        Derive generated feature set $\mathcal{\hat{F}}_t$ by:\\
	        $\mathcal{\hat{F}}_t = \mathcal{F}_{i,t} \cup \mathcal{F}^g_t$;\\
	        
	        \If{$V_A(\mathcal{\hat{F}}_t|y) > V_A(\mathcal{F}^{*}|y)$}{$\mathcal{F}^{*}$ = $\mathcal{\hat{F}}_t$;}
	        
	        Derive $s^1_{t+1} = Rep(\mathcal{\hat{F}}_t)$;\\
	        $\mathcal{R}^1(s^1_t,a^1_t) = U(\mathcal{\hat{F}}_t|y)$;\\
	        Store ($s^1_{t}, a^1_t, \mathcal{R}^1(s^1_t,a^1_t), s^1_{t+1}$) to $\mathcal{D}^1$;\\

	        Derive $s^o_{t+1} = Rep(\mathcal{\hat{F}}_t) \oplus Rep(\mathcal{C}^1_t)$;\\
            $\mathcal{R}^1(s^1_t,a^1_t) = U(\mathcal{\hat{F}}_t|y) - U(\mathcal{F}_t|y)$;\\
            Store ($s^o_{t}, a^o_t, \mathcal{R}^o(s^o_t,a^o_t), s^o_{t+1}$) to $\mathcal{D}^o$;\\
            
            Derive $s^2_{t+1} =
            Rep(\mathcal{\hat{F}}_t) \oplus Rep(\mathcal{C}^1_t) \oplus (o_t)$;\\
            $\mathcal{R}^2(s^2_t,a^2_t) = U(\mathcal{\hat{F}}_t|y) - U(\mathcal{F}_t|y) + V_A(\mathcal{\hat{F}}_t, y)$;\\
            Store ($s^2_{t}, a^2_t, \mathcal{R}^2(s^2_t,a^2_t), s^2_{t+1}$) to $\mathcal{D}^2$;\\
            
            Sample a batch of tuples by prioritized experience replay from $\mathcal{D}^1$,$\mathcal{D}^o$, $\mathcal{D}^2$ respectively to train $Q^1,Q^o,Q^2$ by performing gradient descent optimization with loss function:
            
            $||Q(s_t,a_t) - (\mathcal{R}(s_t, a_t) + \gamma * \text{max}_{a_{t+1}}Q_(s_{t+1},a_{t+1}))||^2$;\\
	        
	        \If{$|\mathcal{\hat{F}}_t| > |\mathcal{F}|*M_{max}$}{$\mathcal{\hat{F}}_t = \text{FEATURE\_SELECTION} (\mathcal{\hat{F}}_{t})$;}
	        
	        Update $\mathcal{F}_{i,t+1} = \mathcal{\hat{F}}_t$;
	    }
	 }
	Return $\mathcal{F}^{*}$.
	\caption{Group-wise Reinforced Feature Generation.}
	\label{grfg_alg}
\end{algorithm}
